# Supplementary material for: SMITIN: Self-Monitored Inference-Time INtervention for Generative Music Transformers
Source: arXiv:2404.02252 source file (2025-02-01)
Supplement: Supplementary file 1 [file probing.tex]

% inst. recognition - drums
\begin{figure}[h]
     \centering
     \subfigure{\includegraphics[height=0.3\textwidth]{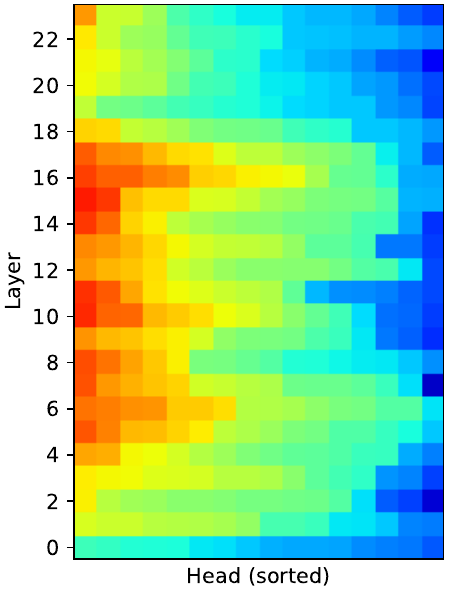}}
     \hfill
     \subfigure{\includegraphics[height=0.3\textwidth]{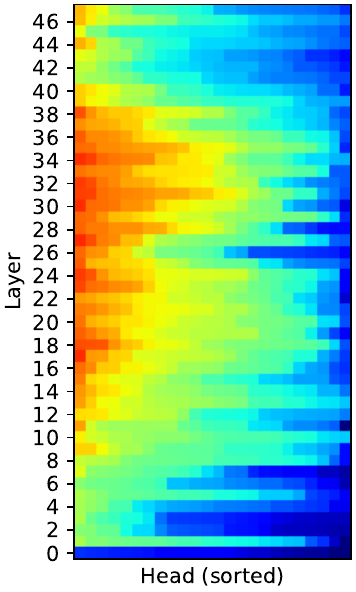}}
     \hfill
     \subfigure{\includegraphics[height=0.3\textwidth]{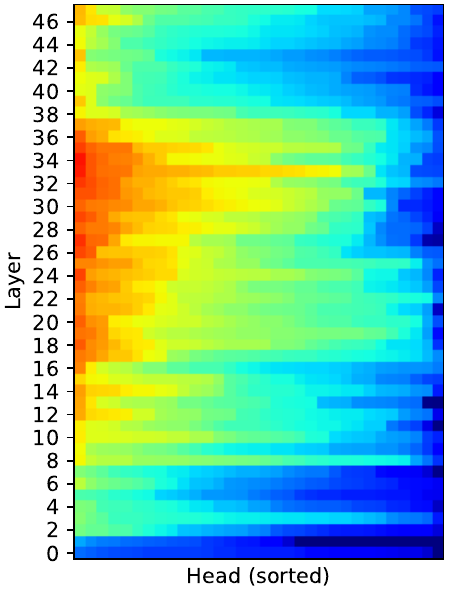}}
     \hfill
     \subfigure{\includegraphics[height=0.3\textwidth]{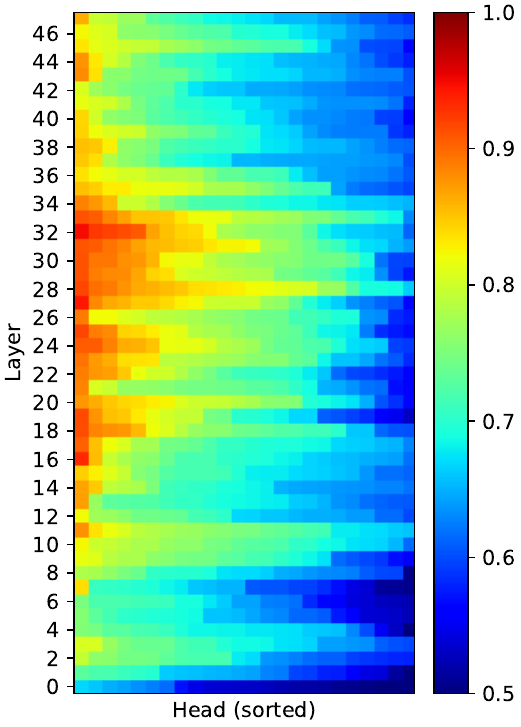}}
     \setcounter{subfigure}{0}
     \subfigure[MusicGen$_\text{small}$]{\includegraphics[width=0.24\textwidth]{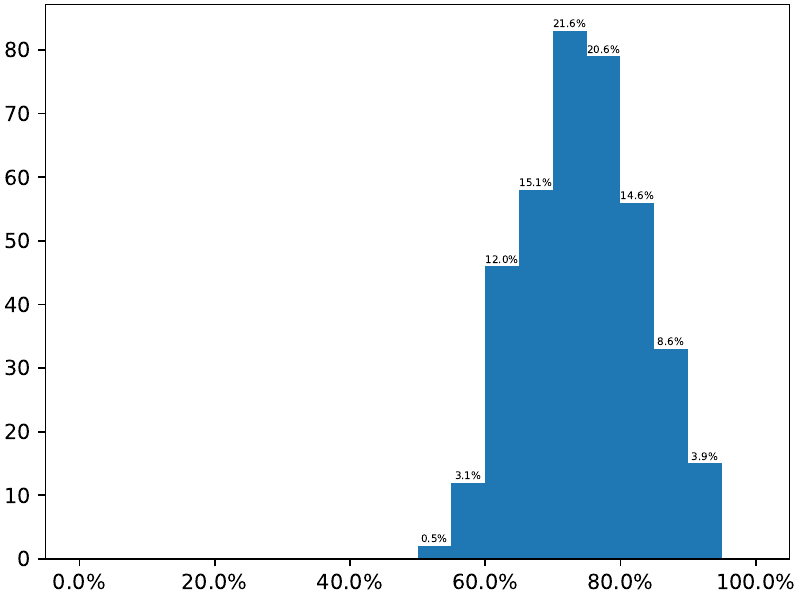}}
     \hfill
     \subfigure[MusicGen$_\text{medium}$]{\includegraphics[width=0.24\textwidth]{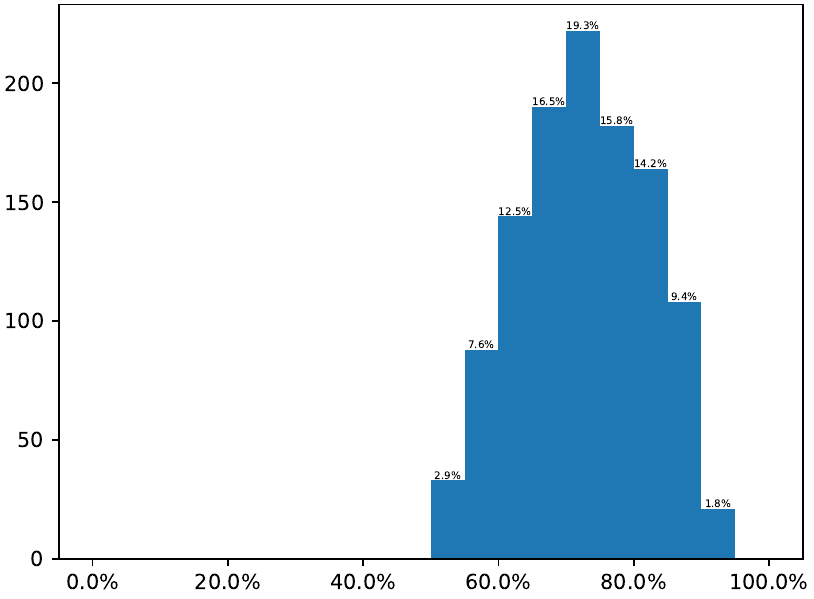}}
     \hfill
     \subfigure[MusicGen$_\text{large}$]{\includegraphics[width=0.24\textwidth]{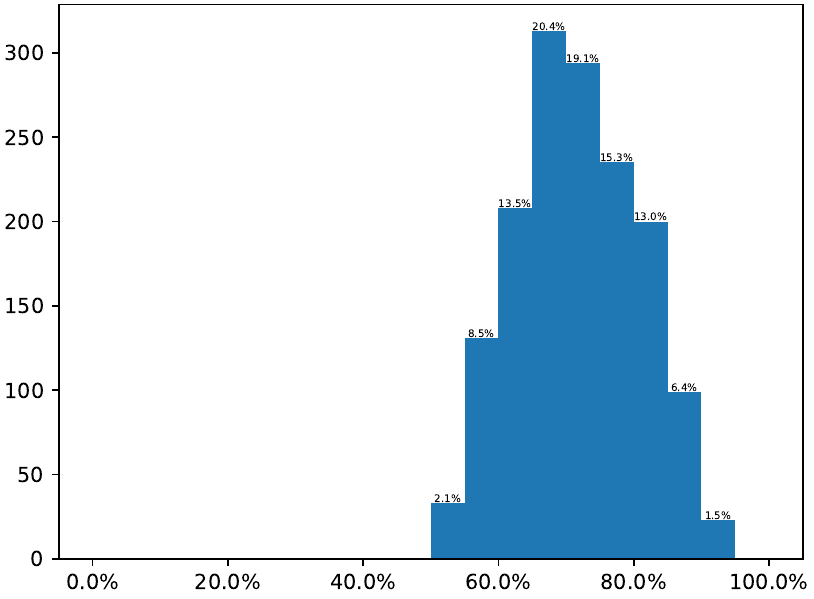}}
     \hfill
     \subfigure[MusicGen$_\text{melody}$]{\includegraphics[width=0.24\textwidth]{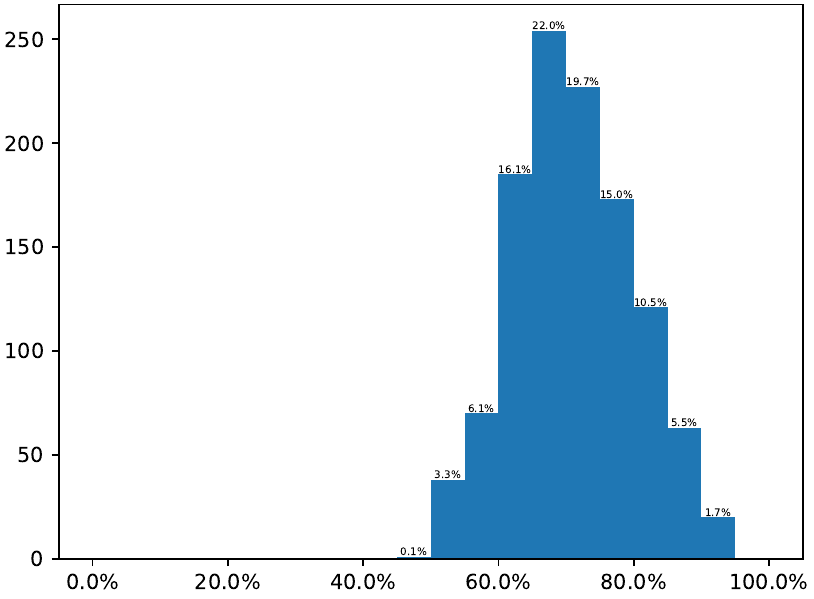}}
     \caption{Probe accuracy and its histogram for instrument recognition: \textit{drums}}
    \label{fig:probe_acc_drums}
\end{figure}

% inst. recognition - bass
\begin{figure}[t]
     \centering
     \subfigure{\includegraphics[height=0.3\textwidth]{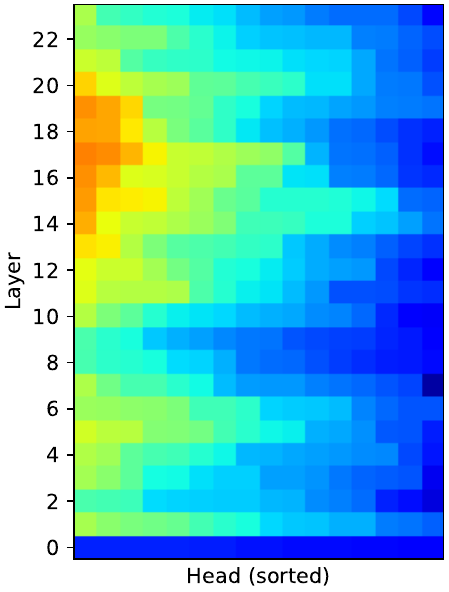}}
     \hfill
     \subfigure{\includegraphics[height=0.3\textwidth]{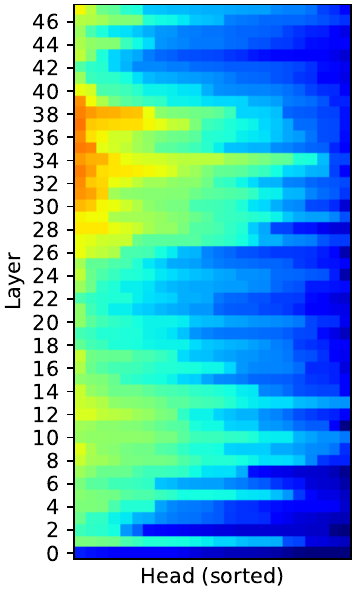}}
     \hfill
     \subfigure{\includegraphics[height=0.3\textwidth]{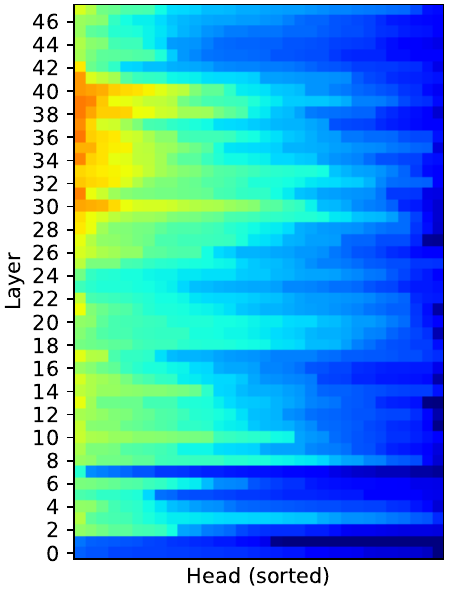}}
     \hfill
     \subfigure{\includegraphics[height=0.3\textwidth]{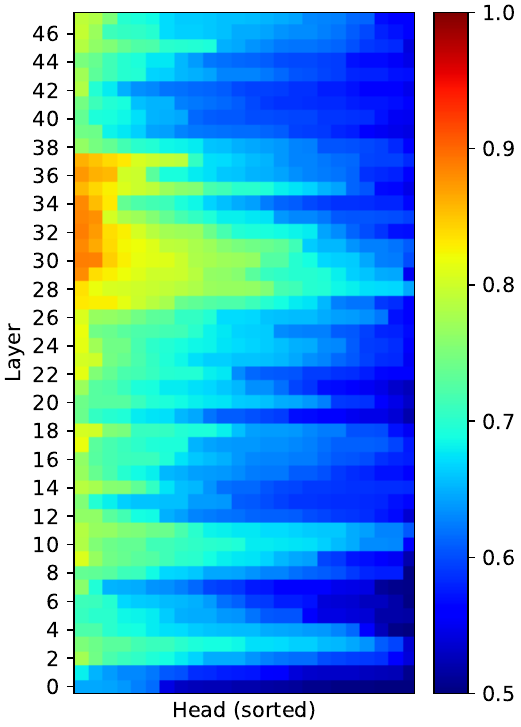}}
     \setcounter{subfigure}{0}
     \subfigure[MusicGen$_\text{small}$]{\includegraphics[width=0.24\textwidth]{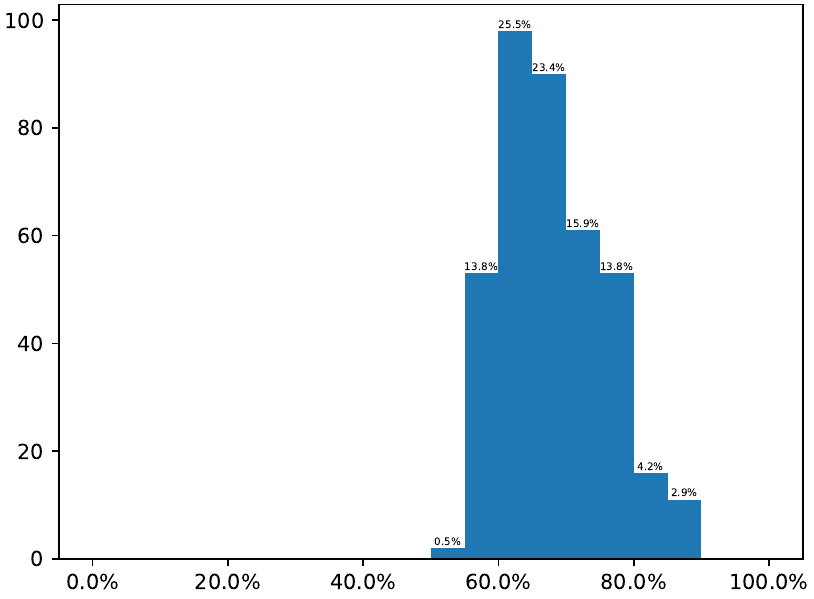}}
     \hfill
     \subfigure[MusicGen$_\text{medium}$]{\includegraphics[width=0.24\textwidth]{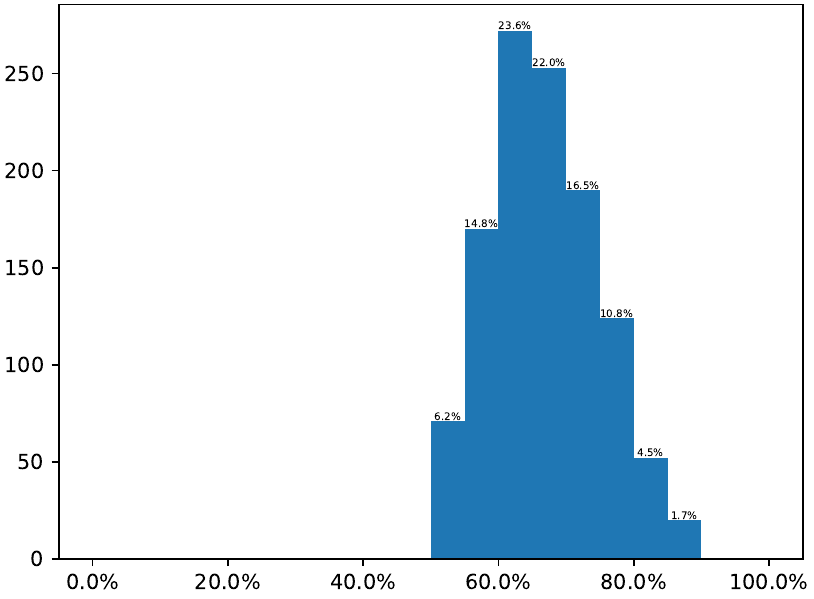}}
     \hfill
     \subfigure[MusicGen$_\text{large}$]{\includegraphics[width=0.24\textwidth]{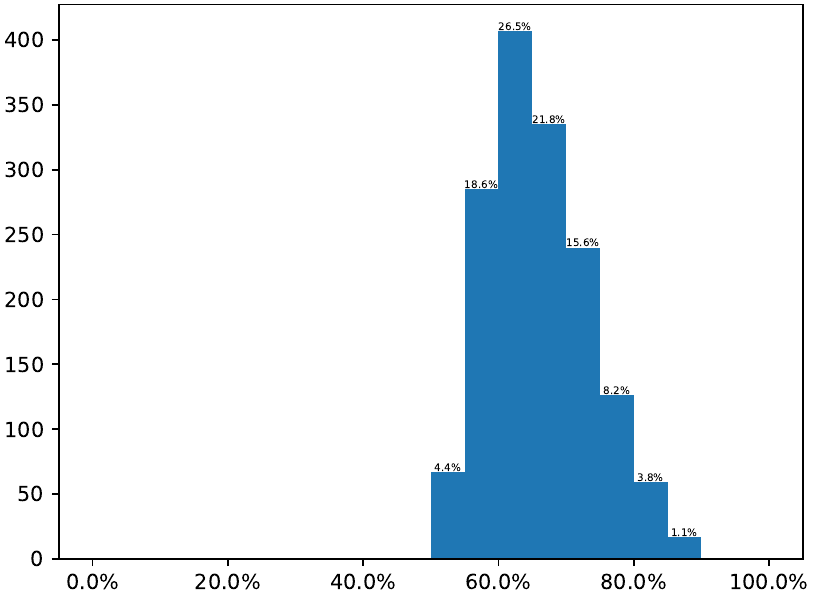}}
     \hfill
     \subfigure[MusicGen$_\text{melody}$]{\includegraphics[width=0.24\textwidth]{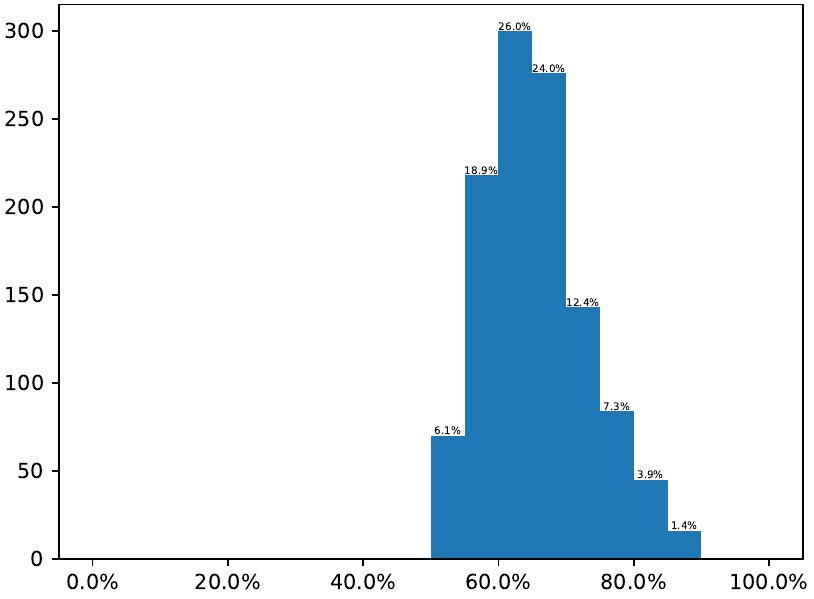}}
     \caption{Probe accuracy and its histogram for instrument recognition: \textit{bass}}
    \label{fig:probe_acc_bass}
\end{figure}

% inst. recognition - guitar
\begin{figure}[t]
     \centering
     \subfigure{\includegraphics[height=0.3\textwidth]{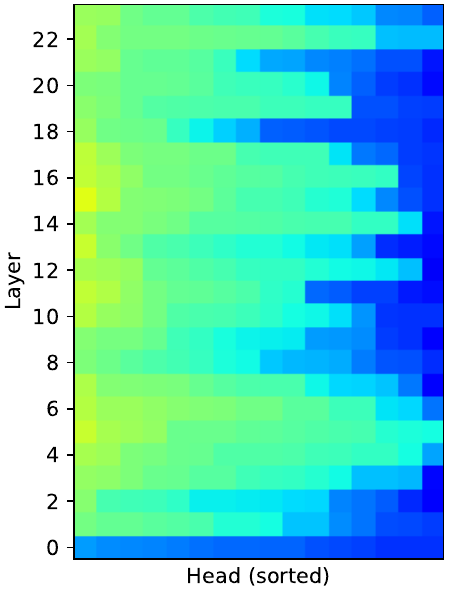}}
     \hfill
     \subfigure{\includegraphics[height=0.3\textwidth]{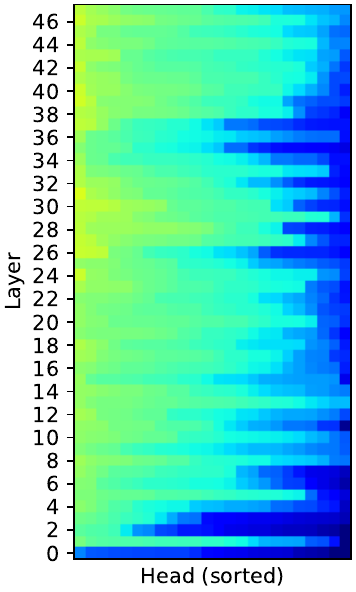}}
     \hfill
     \subfigure{\includegraphics[height=0.3\textwidth]{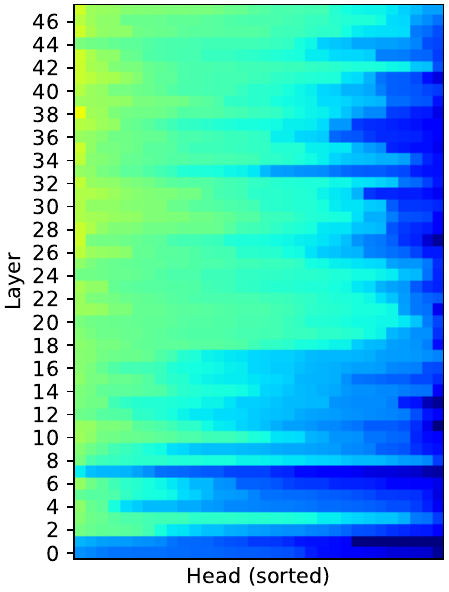}}
     \hfill
     \subfigure{\includegraphics[height=0.3\textwidth]{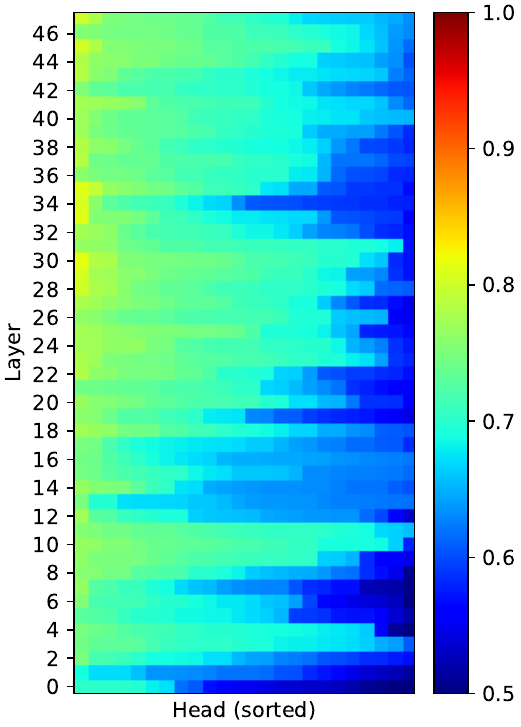}}
     \setcounter{subfigure}{0}
     \subfigure[MusicGen$_\text{small}$]{\includegraphics[width=0.24\textwidth]{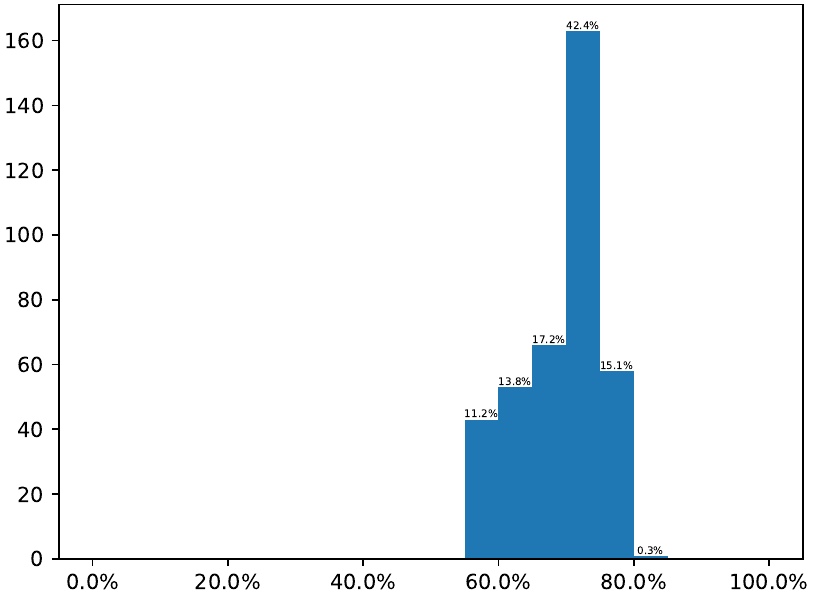}}
     \hfill
     \subfigure[MusicGen$_\text{medium}$]{\includegraphics[width=0.24\textwidth]{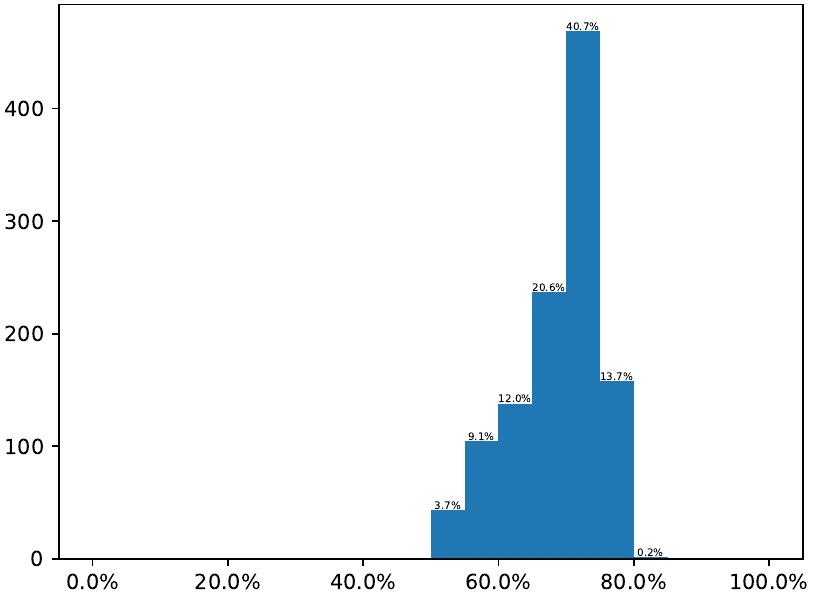}}
     \hfill
     \subfigure[MusicGen$_\text{large}$]{\includegraphics[width=0.24\textwidth]{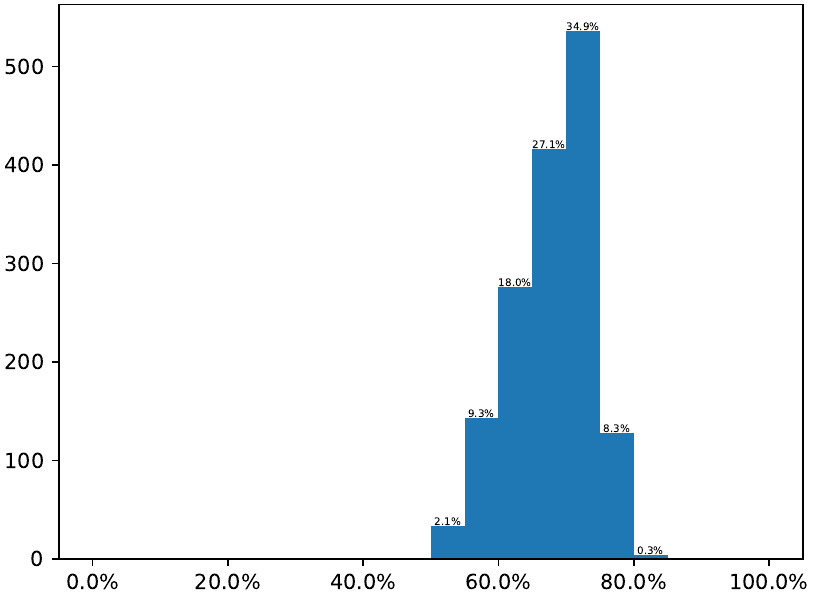}}
     \hfill
     \subfigure[MusicGen$_\text{melody}$]{\includegraphics[width=0.24\textwidth]{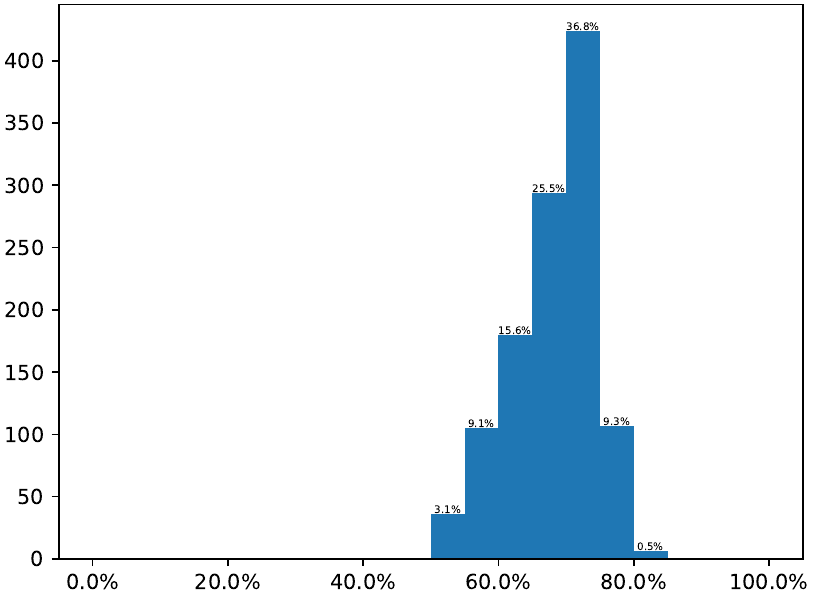}}
     \caption{Probe accuracy and its histogram for instrument recognition: \textit{guitar}}
    \label{fig:probe_acc_guitar}
\end{figure}

% inst. recognition - piano
\begin{figure}[t]
     \centering
     \subfigure{\includegraphics[height=0.3\textwidth]{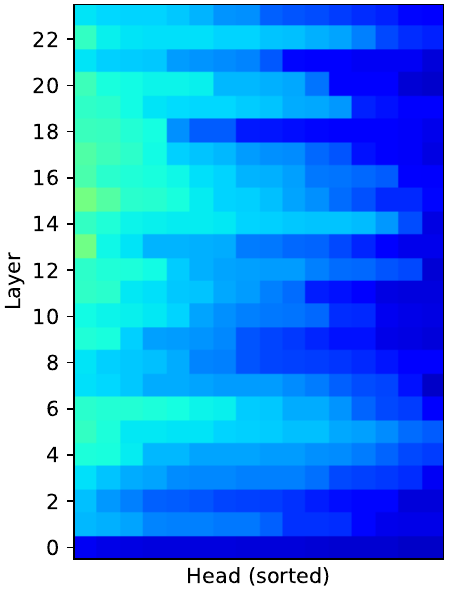}}
     \hfill
     \subfigure{\includegraphics[height=0.3\textwidth]{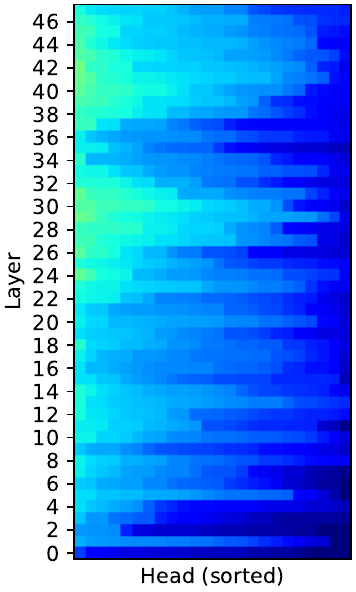}}
     \hfill
     \subfigure{\includegraphics[height=0.3\textwidth]{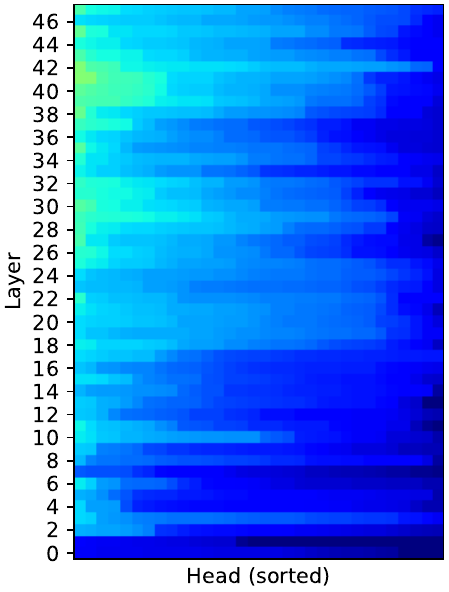}}
     \hfill
     \subfigure{\includegraphics[height=0.3\textwidth]{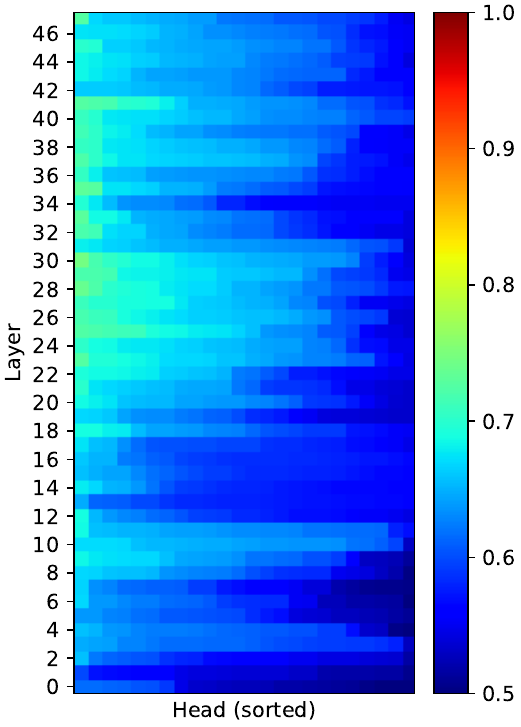}}
     \setcounter{subfigure}{0}
     \subfigure[MusicGen$_\text{small}$]{\includegraphics[width=0.24\textwidth]{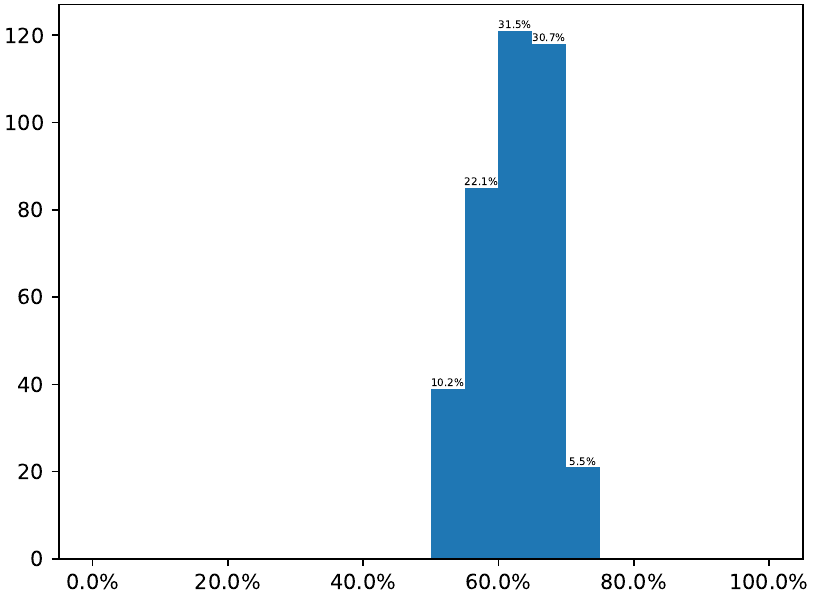}}
     \hfill
     \subfigure[MusicGen$_\text{medium}$]{\includegraphics[width=0.24\textwidth]{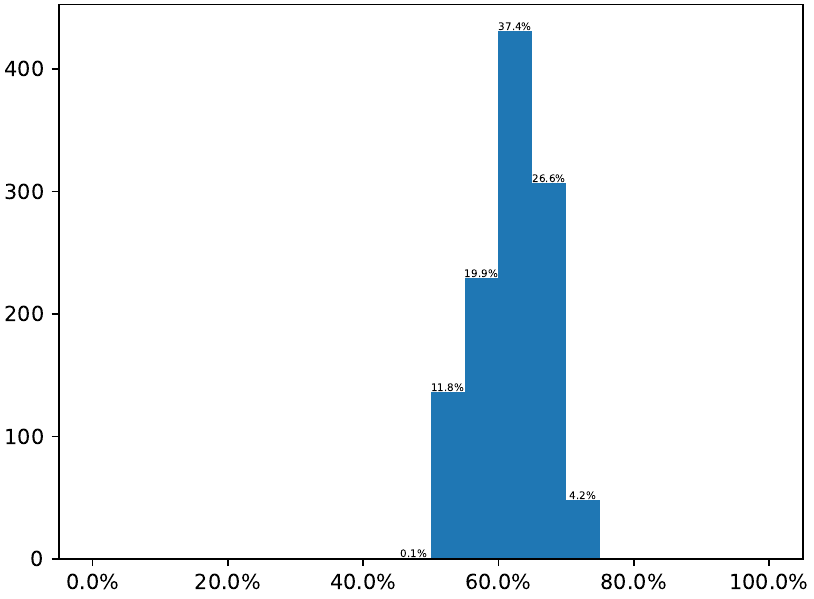}}
     \hfill
     \subfigure[MusicGen$_\text{large}$]{\includegraphics[width=0.24\textwidth]{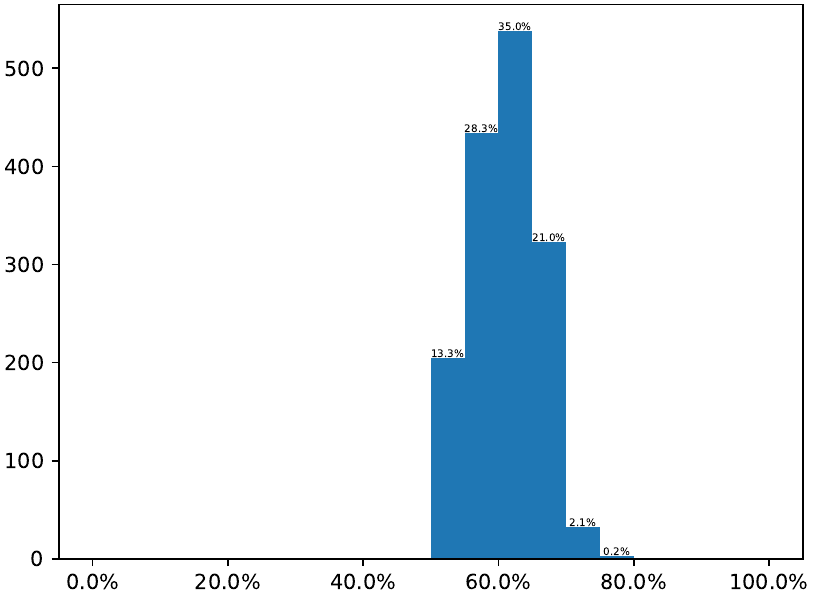}}
     \hfill
     \subfigure[MusicGen$_\text{melody}$]{\includegraphics[width=0.24\textwidth]{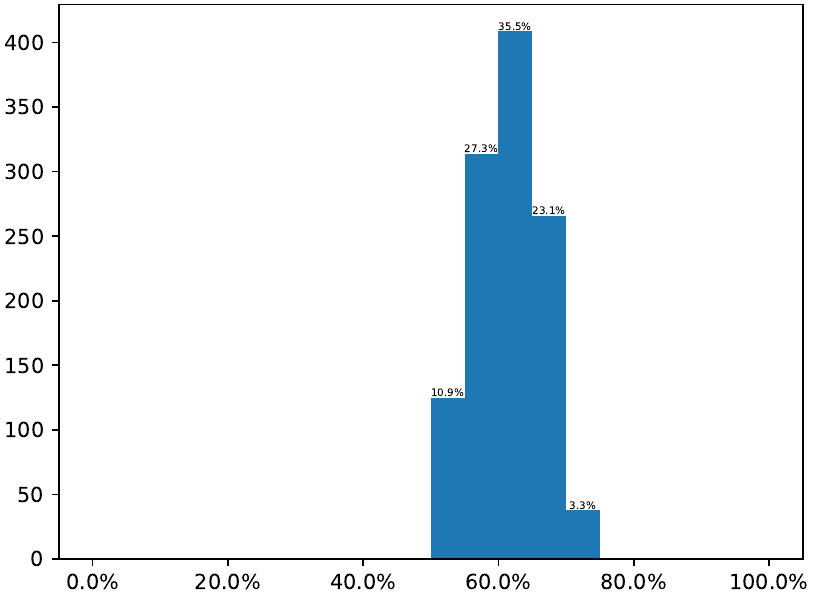}}
     \caption{Probe accuracy and its histogram for instrument recognition: \textit{piano}}
    \label{fig:probe_acc_piano}
\end{figure}

% music tagging - AUC
\begin{figure}[t]
     \centering
     \subfigure{\includegraphics[height=0.3\textwidth]{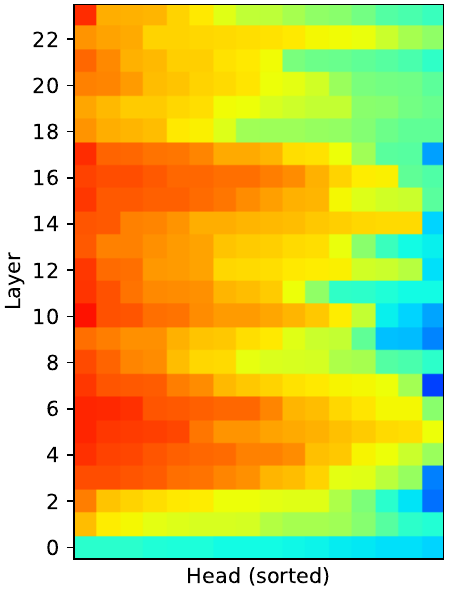}}
     \hfill
     \subfigure{\includegraphics[height=0.3\textwidth]{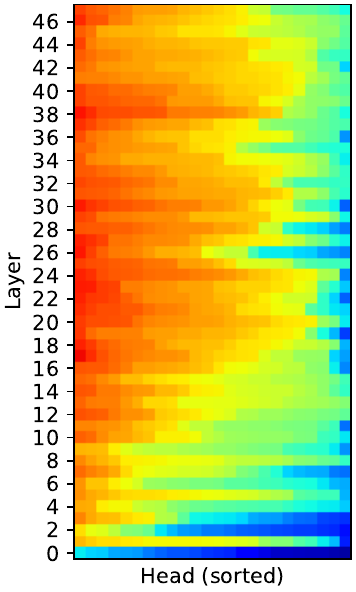}}
     \hfill
     \subfigure{\includegraphics[height=0.3\textwidth]{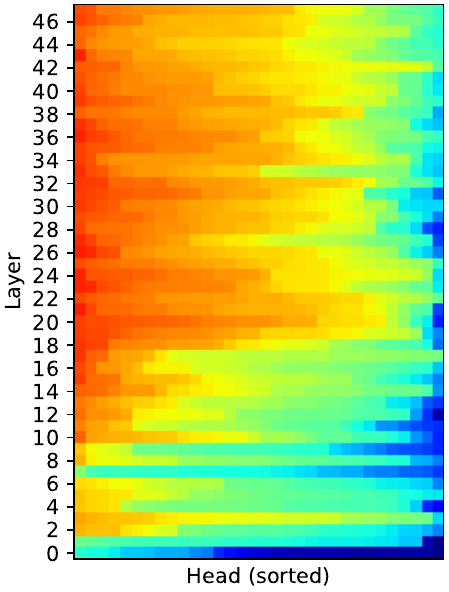}}
     \hfill
     \subfigure{\includegraphics[height=0.3\textwidth]{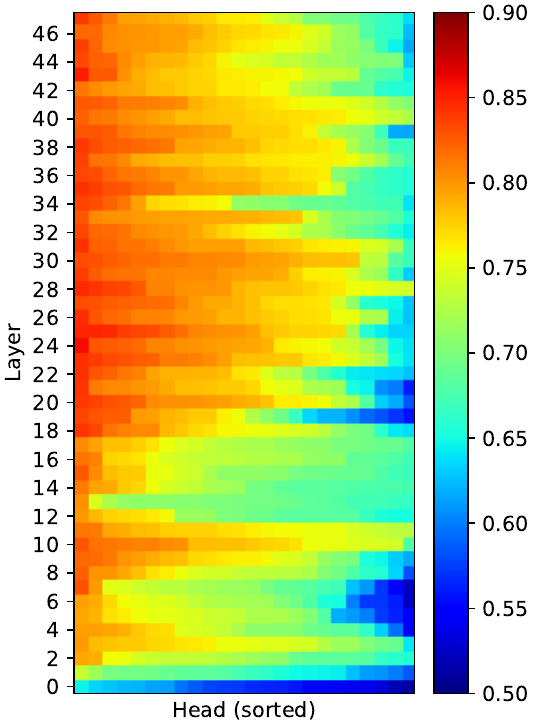}}
     \setcounter{subfigure}{0}
     \subfigure[MusicGen$_\text{small}$]{\includegraphics[width=0.24\textwidth]{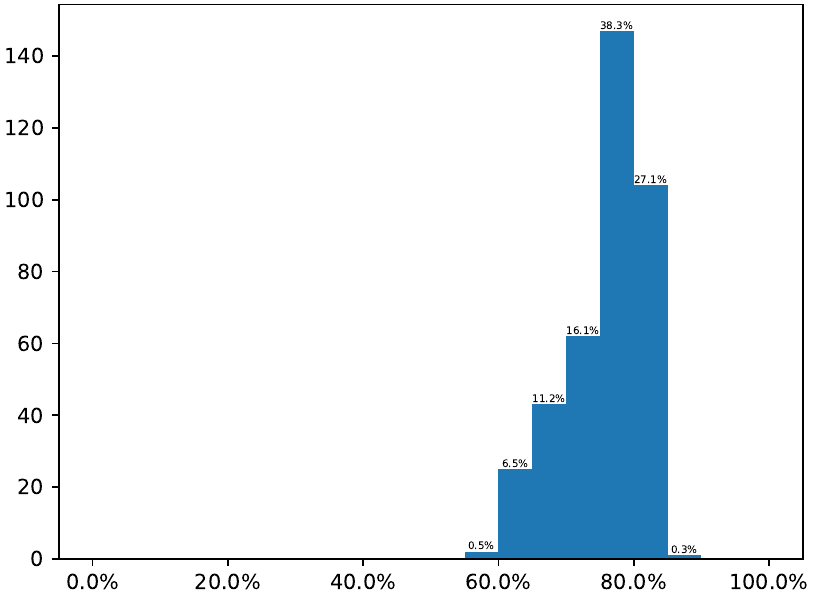}}
     \hfill
     \subfigure[MusicGen$_\text{medium}$]{\includegraphics[width=0.24\textwidth]{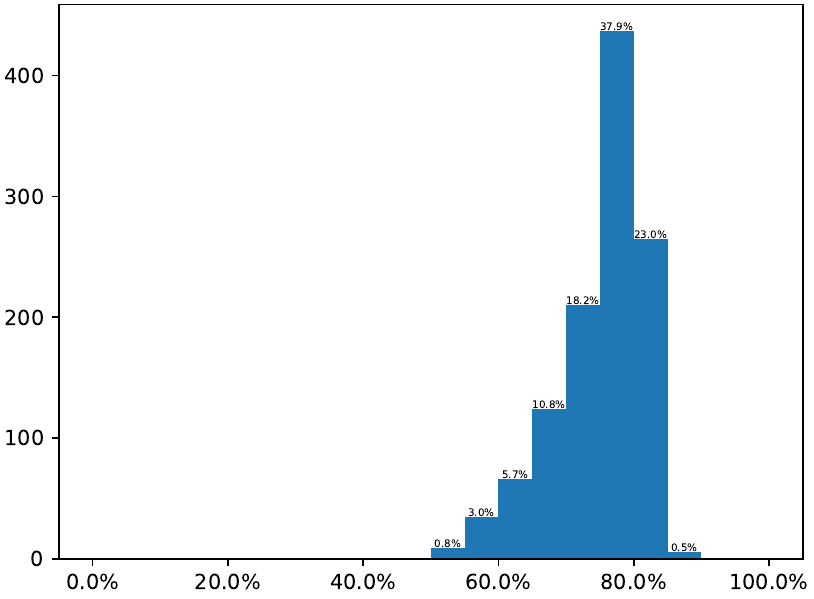}}
     \hfill
     \subfigure[MusicGen$_\text{large}$]{\includegraphics[width=0.24\textwidth]{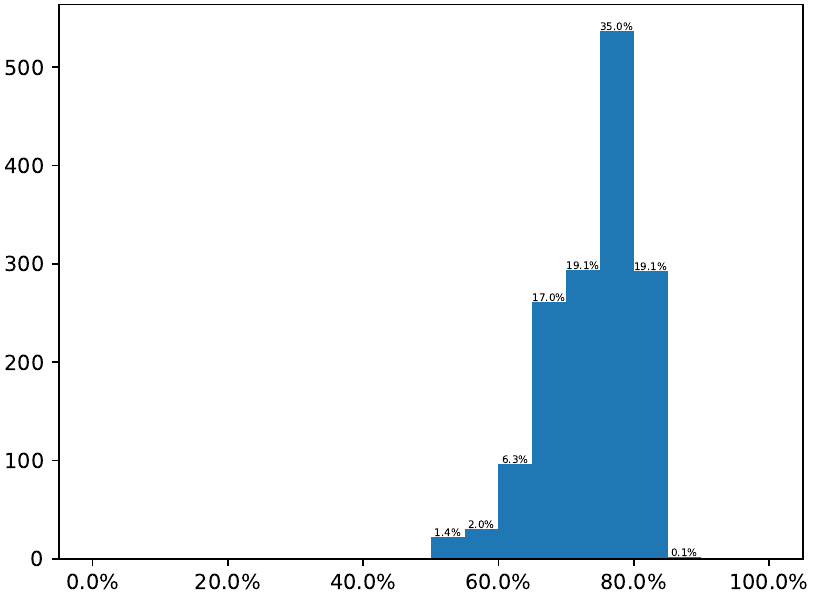}}
     \hfill
     \subfigure[MusicGen$_\text{melody}$]{\includegraphics[width=0.24\textwidth]{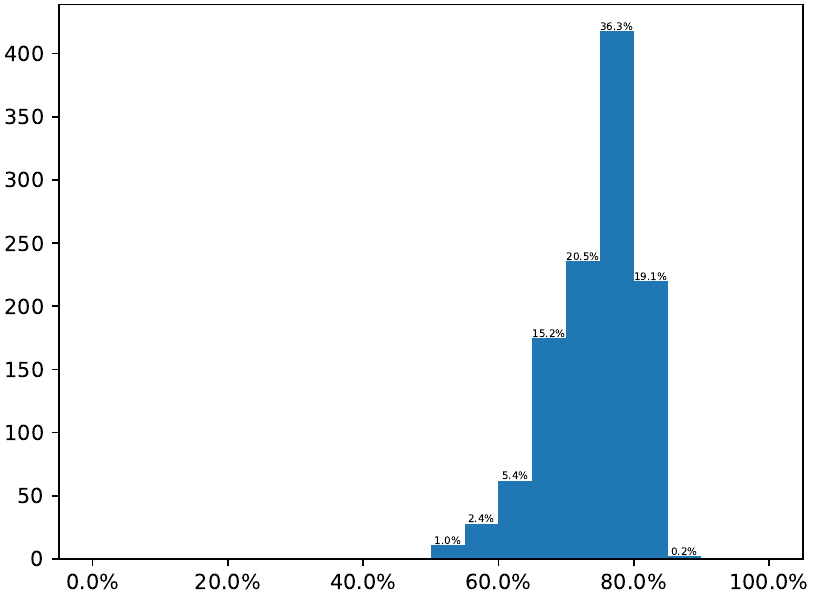}}
     \caption{Probe accuracy and its histogram for music tagging on MTT (AUC)}
    \label{fig:probe_acc_tagging_auc}
\end{figure}

% music tagging - AP
\begin{figure}[t]
     \centering
     \subfigure{\includegraphics[height=0.3\textwidth]{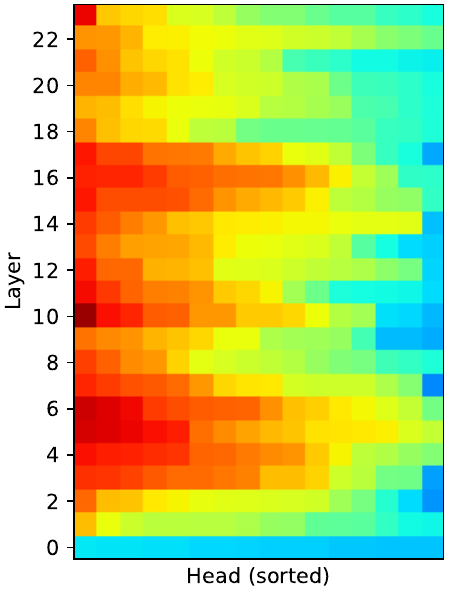}}
     \hfill
     \subfigure{\includegraphics[height=0.3\textwidth]{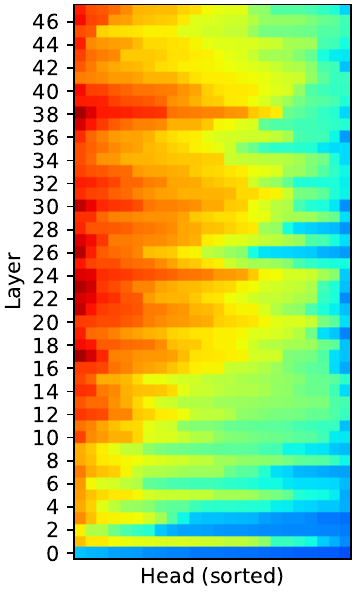}}
     \hfill
     \subfigure{\includegraphics[height=0.3\textwidth]{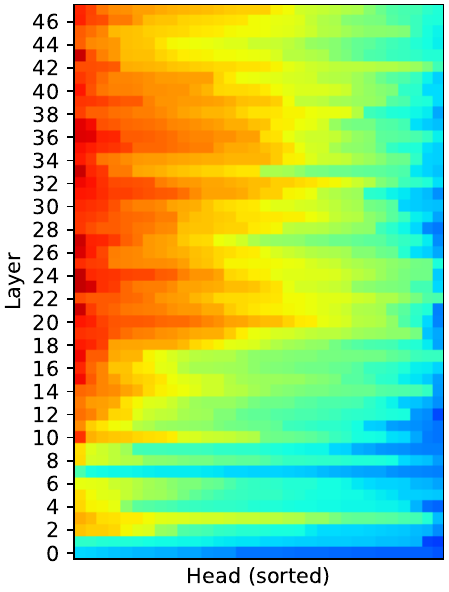}}
     \hfill
     \subfigure{\includegraphics[height=0.3\textwidth]{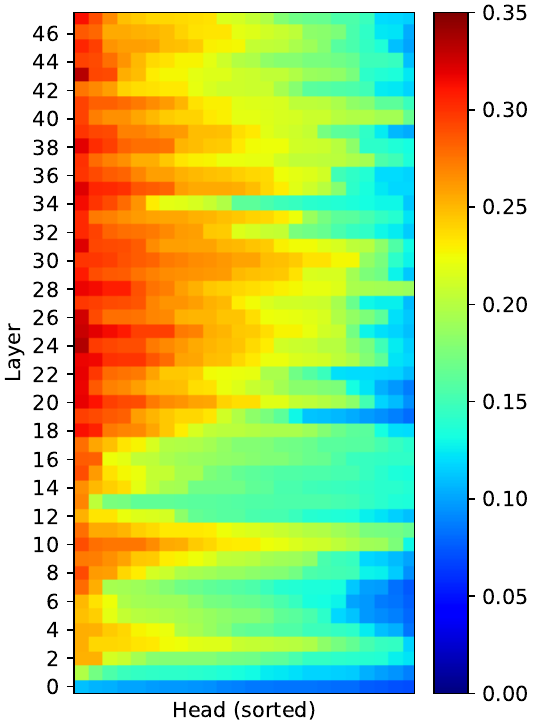}}
     \setcounter{subfigure}{0}
     \subfigure[MusicGen$_\text{small}$]{\includegraphics[width=0.24\textwidth]{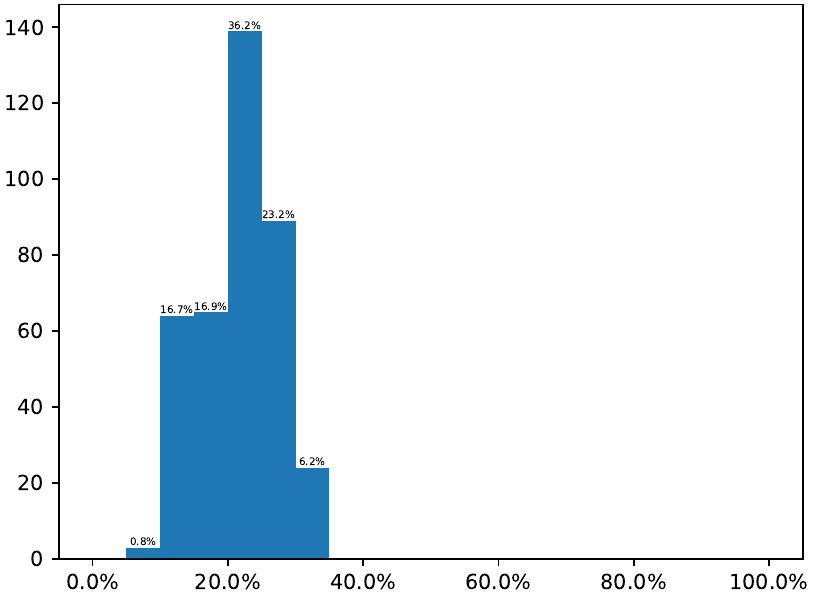}}
     \hfill
     \subfigure[MusicGen$_\text{medium}$]{\includegraphics[width=0.24\textwidth]{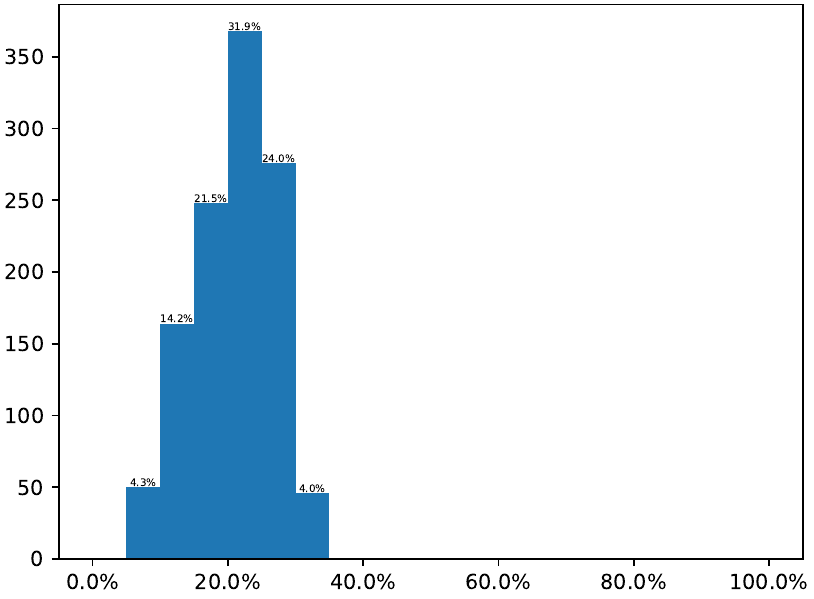}}
     \hfill
     \subfigure[MusicGen$_\text{large}$]{\includegraphics[width=0.24\textwidth]{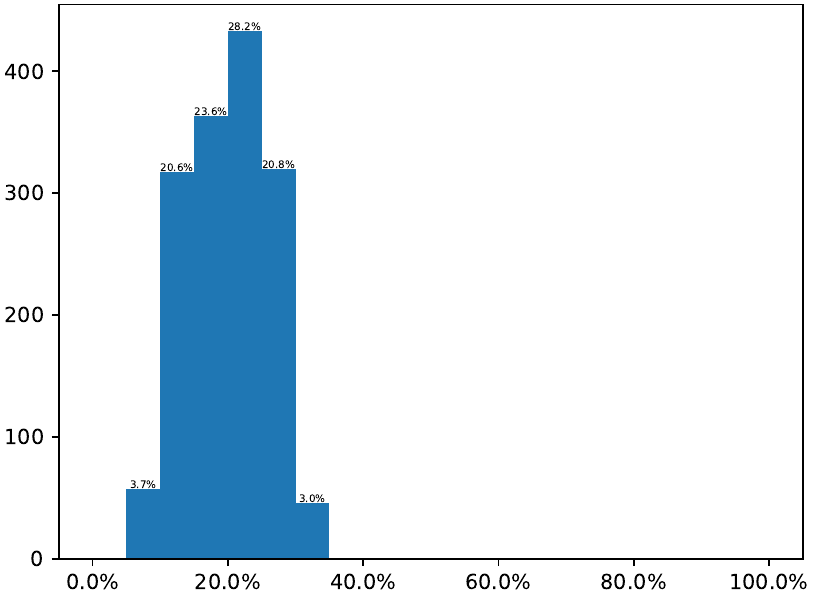}}
     \hfill
     \subfigure[MusicGen$_\text{melody}$]{\includegraphics[width=0.24\textwidth]{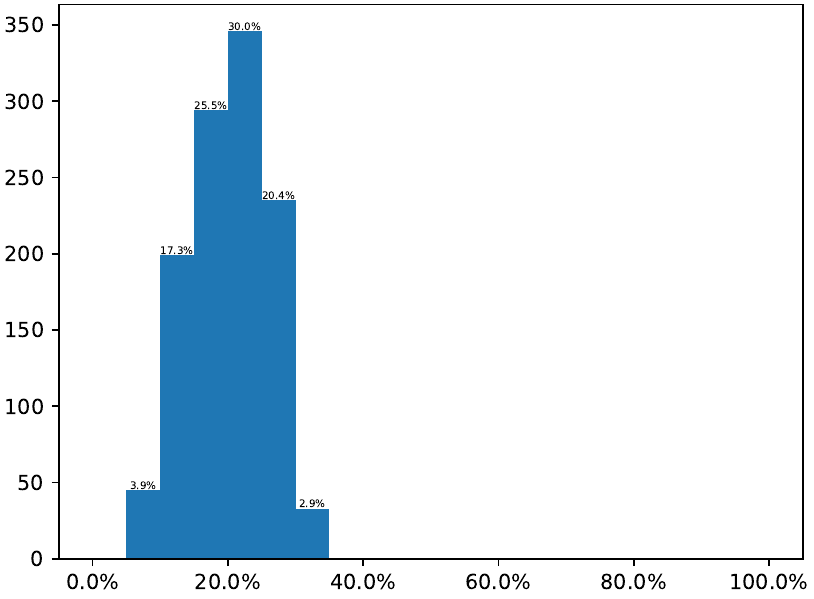}}
     \caption{Probe accuracy and its histogram for music tagging on MTT (AP)}
    \label{fig:probe_acc_tagging_ap}
\end{figure}

% genre classification
\begin{figure}[t]
     \centering
     \subfigure{\includegraphics[height=0.3\textwidth]{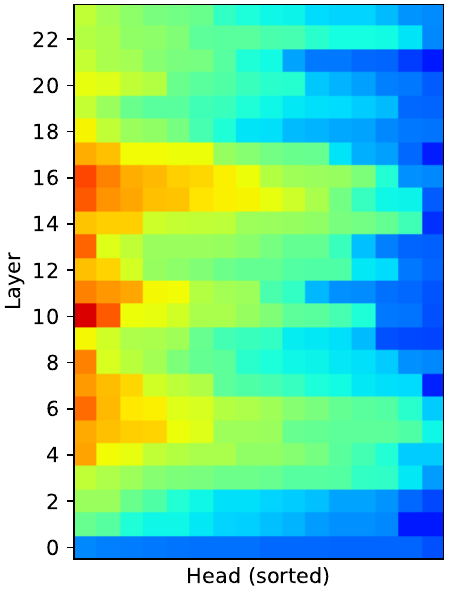}}
     \hfill
     \subfigure{\includegraphics[height=0.3\textwidth]{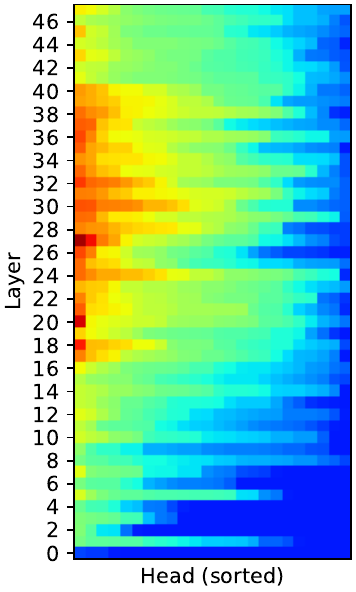}}
     \hfill
     \subfigure{\includegraphics[height=0.3\textwidth]{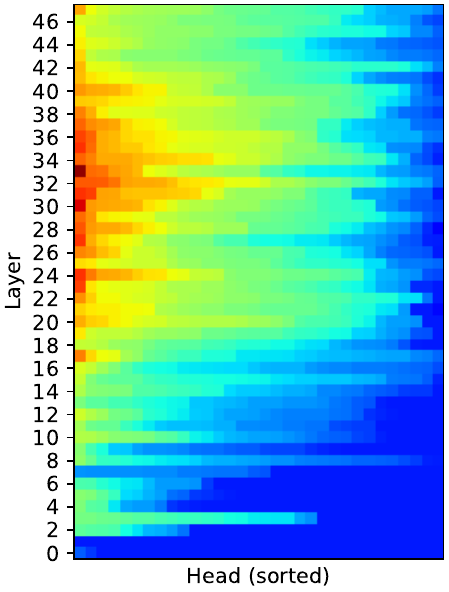}}
     \hfill
     \subfigure{\includegraphics[height=0.3\textwidth]{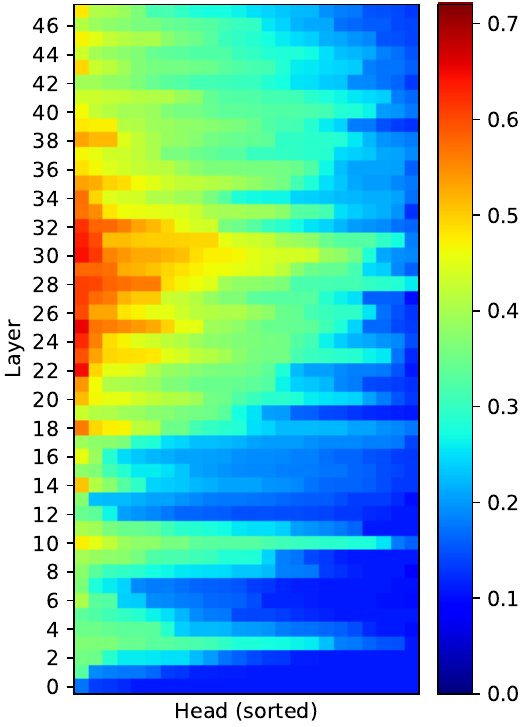}}
     \setcounter{subfigure}{0}
     \subfigure[MusicGen$_\text{small}$]{\includegraphics[width=0.24\textwidth]{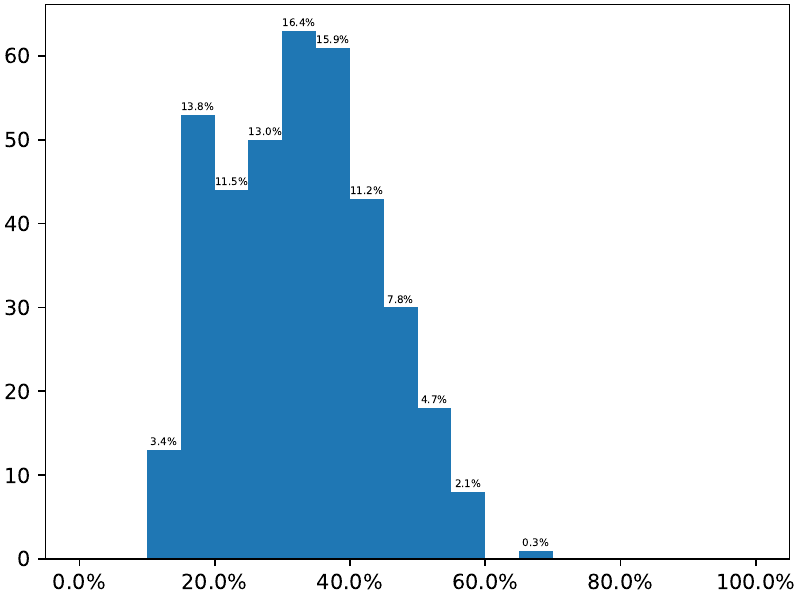}}
     \hfill
     \subfigure[MusicGen$_\text{medium}$]{\includegraphics[width=0.24\textwidth]{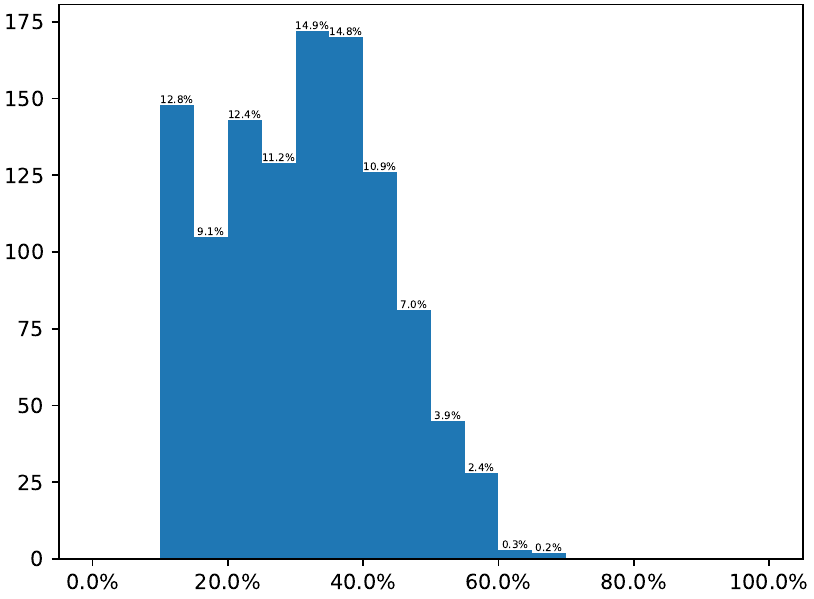}}
     \hfill
     \subfigure[MusicGen$_\text{large}$]{\includegraphics[width=0.24\textwidth]{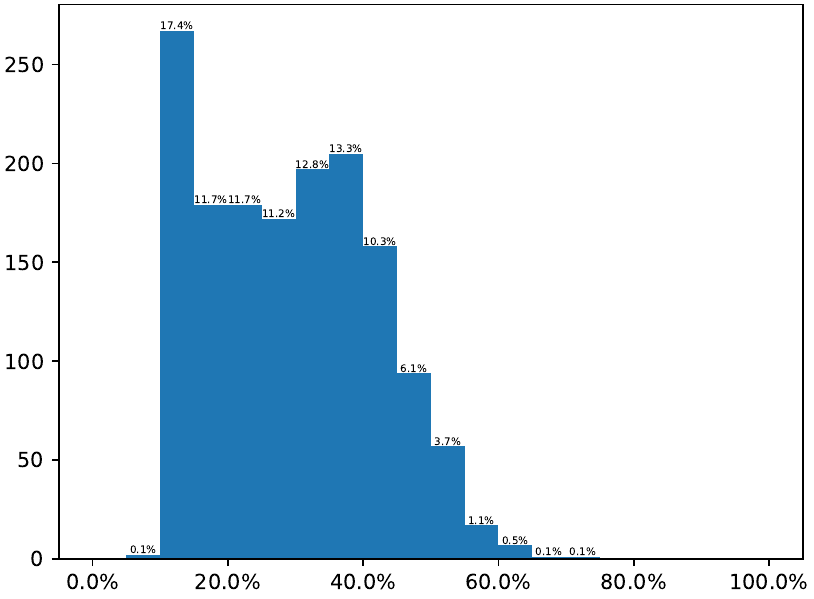}}
     \hfill
     \subfigure[MusicGen$_\text{melody}$]{\includegraphics[width=0.24\textwidth]{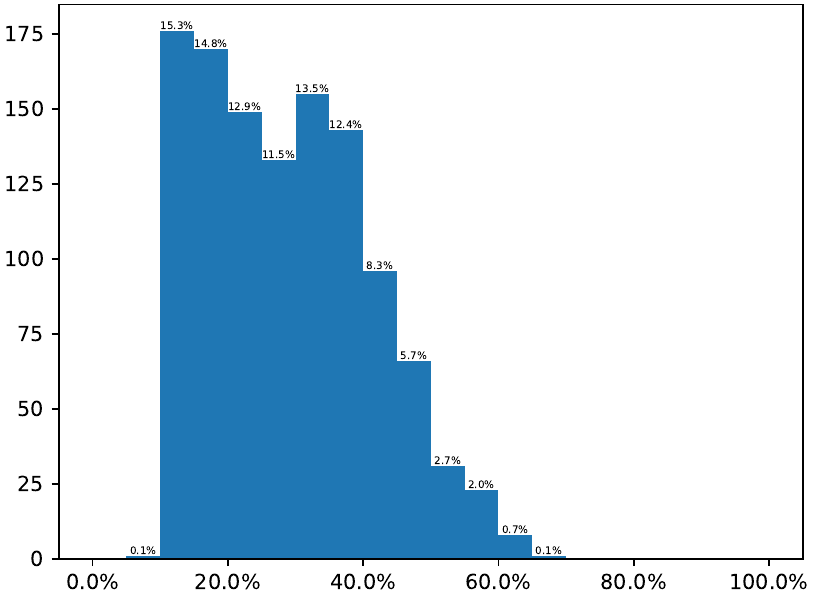}}
     \caption{Probe accuracy and its histogram for genre classification on GTZAN}
    \label{fig:probe_acc_genre_classification}
\end{figure}

% key detection
\begin{figure}[t]
     \centering
     \subfigure{\includegraphics[height=0.3\textwidth]{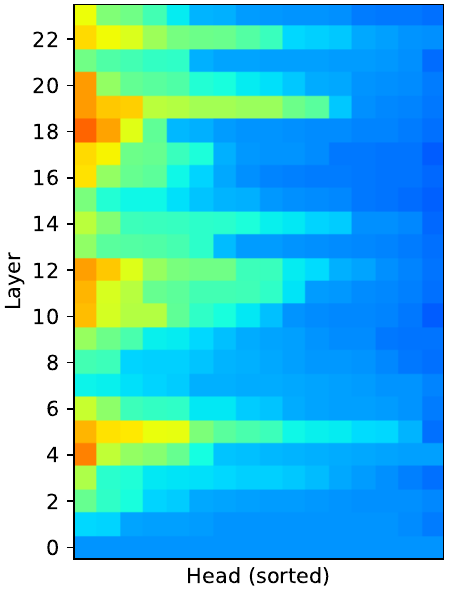}}
     \hfill
     \subfigure{\includegraphics[height=0.3\textwidth]{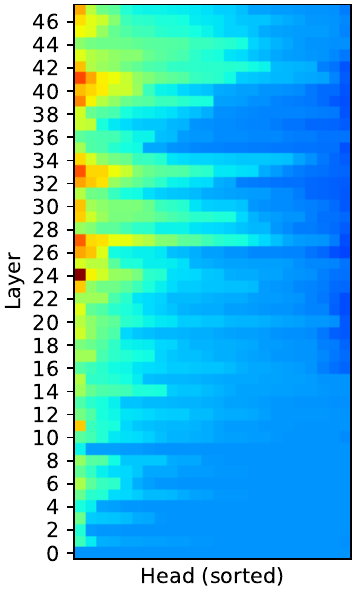}}
     \hfill
     \subfigure{\includegraphics[height=0.3\textwidth]{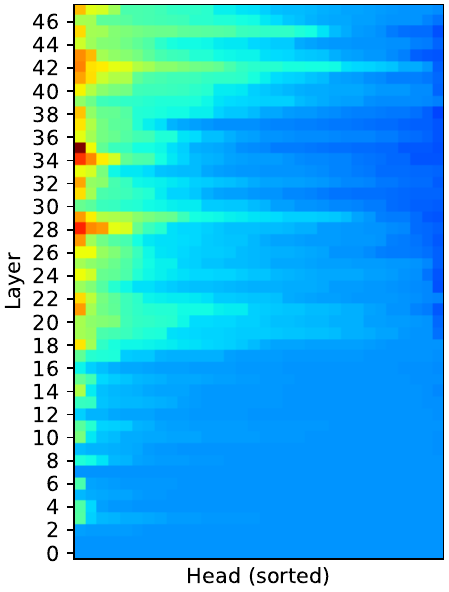}}
     \hfill
     \subfigure{\includegraphics[height=0.3\textwidth]{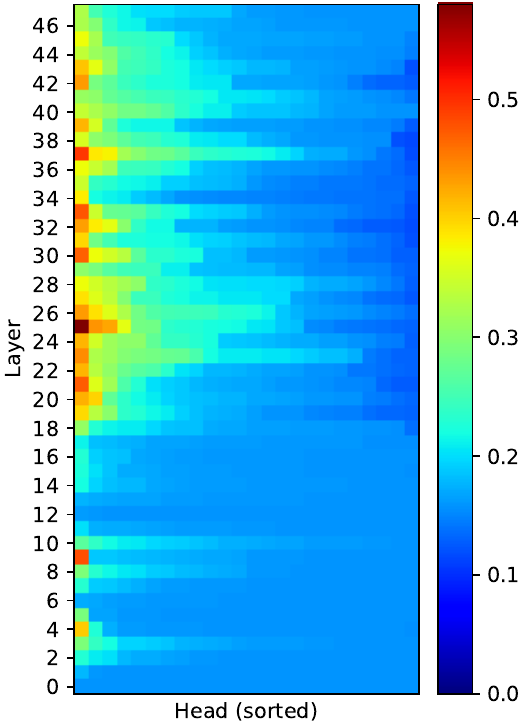}}
     \setcounter{subfigure}{0}
     \subfigure[MusicGen$_\text{small}$]{\includegraphics[width=0.24\textwidth]{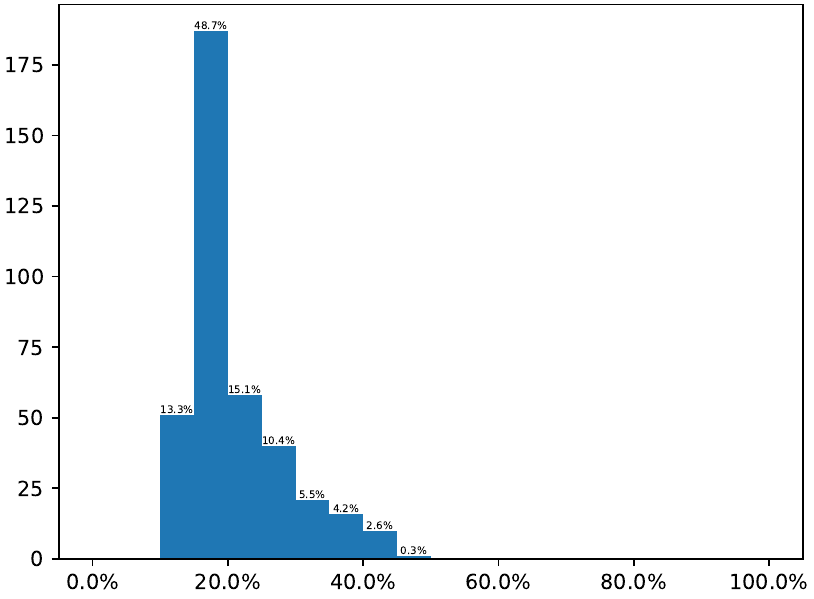}}
     \hfill
     \subfigure[MusicGen$_\text{medium}$]{\includegraphics[width=0.24\textwidth]{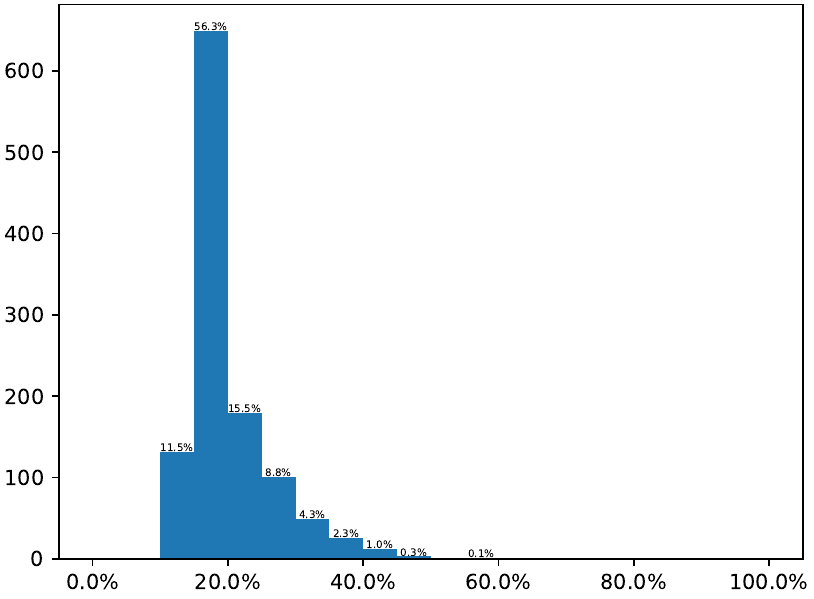}}
     \hfill
     \subfigure[MusicGen$_\text{large}$]{\includegraphics[width=0.24\textwidth]{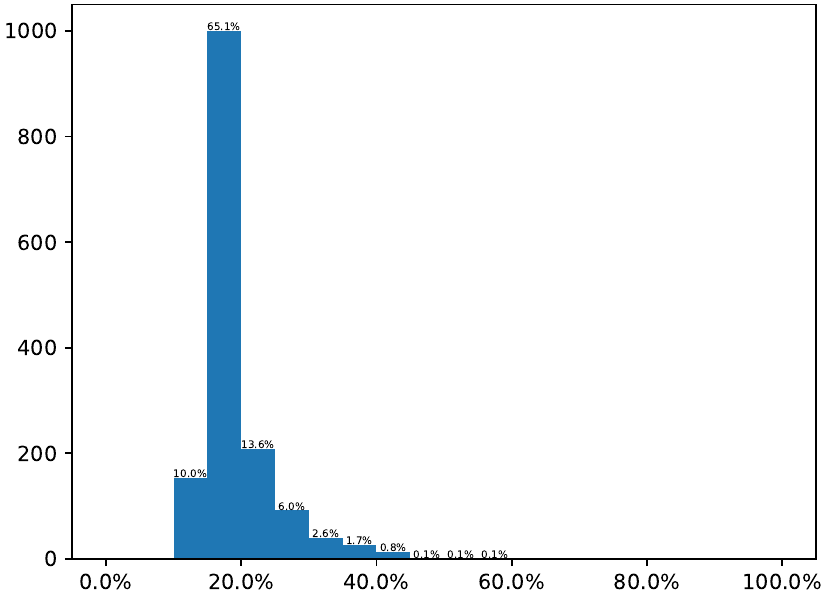}}
     \hfill
     \subfigure[MusicGen$_\text{melody}$]{\includegraphics[width=0.24\textwidth]{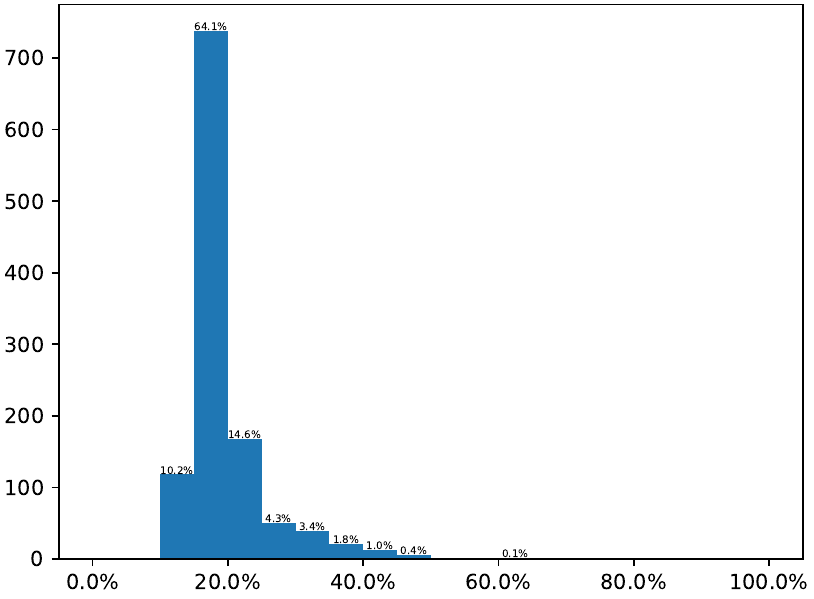}}
     \caption{Probe accuracy and its histogram for key detection on GiantSteps}
    \label{fig:probe_acc_key_detection}
\end{figure}

% emotion recognition - R2^A
\begin{figure}[t]
     \centering
     \subfigure{\includegraphics[height=0.3\textwidth]{figs/probes_accuracies/emotion_recognition/R2^A/small_avg_arousal_r2_scaled.pdf}}
     \hfill
     \subfigure{\includegraphics[height=0.3\textwidth]{figs/probes_accuracies/emotion_recognition/R2^A/medium_avg_arousal_r2.pdf}}
     \hfill
     \subfigure{\includegraphics[height=0.3\textwidth]{figs/probes_accuracies/emotion_recognition/R2^A/large_avg_arousal_r2_scaled.pdf}}
     \hfill
     \subfigure{\includegraphics[height=0.3\textwidth]{figs/probes_accuracies/emotion_recognition/R2^A/melody_avg_arousal_r2_scaled.pdf}}
     \setcounter{subfigure}{0}
     \subfigure[MusicGen$_\text{small}$]{\includegraphics[width=0.24\textwidth]{figs/probes_accuracies/emotion_recognition/R2^A/small_avg_probes_hist_arousal_r2.pdf}}
     \hfill
     \subfigure[MusicGen$_\text{medium}$]{\includegraphics[width=0.24\textwidth]{figs/probes_accuracies/emotion_recognition/R2^A/medium_avg_probes_hist_arousal_r2.pdf}}
     \hfill
     \subfigure[MusicGen$_\text{large}$]{\includegraphics[width=0.24\textwidth]{figs/probes_accuracies/emotion_recognition/R2^A/large_avg_probes_hist_arousal_r2.pdf}}
     \hfill
     \subfigure[MusicGen$_\text{melody}$]{\includegraphics[width=0.24\textwidth]{figs/probes_accuracies/emotion_recognition/R2^A/melody_avg_probes_hist_arousal_r2.pdf}}
     \caption{Probe accuracy and its histogram for emotion recognition (R2$^A$)}
    \label{fig:probe_acc_emotion_recognition_arousal}
\end{figure}

% emotion recognition - R2^V
\begin{figure}[t]
     \centering
     \subfigure{\includegraphics[height=0.3\textwidth]{figs/probes_accuracies/emotion_recognition/R2^V/small_avg_valence_r2_scaled.pdf}}
     \hfill
     \subfigure{\includegraphics[height=0.3\textwidth]{figs/probes_accuracies/emotion_recognition/R2^V/medium_avg_valence_r2_scaled.pdf}}
     \hfill
     \subfigure{\includegraphics[height=0.3\textwidth]{figs/probes_accuracies/emotion_recognition/R2^V/large_avg_valence_r2_scaled.pdf}}
     \hfill
     \subfigure{\includegraphics[height=0.3\textwidth]{figs/probes_accuracies/emotion_recognition/R2^V/melody_avg_valence_r2_scaled.pdf}}
     \setcounter{subfigure}{0}
     \subfigure[MusicGen$_\text{small}$]{\includegraphics[width=0.24\textwidth]{figs/probes_accuracies/emotion_recognition/R2^V/small_avg_probes_hist_valence_r2.pdf}}
     \hfill
     \subfigure[MusicGen$_\text{medium}$]{\includegraphics[width=0.24\textwidth]{figs/probes_accuracies/emotion_recognition/R2^V/medium_avg_probes_hist_valence_r2.pdf}}
     \hfill
     \subfigure[MusicGen$_\text{large}$]{\includegraphics[width=0.24\textwidth]{figs/probes_accuracies/emotion_recognition/R2^V/large_avg_probes_hist_valence_r2.pdf}}
     \hfill
     \subfigure[MusicGen$_\text{melody}$]{\includegraphics[width=0.24\textwidth]{figs/probes_accuracies/emotion_recognition/R2^V/melody_avg_probes_hist_valence_r2.pdf}}
     \caption{Probe accuracy and its histogram for emotion recognition (R2$^V$)}
    \label{fig:probe_acc_emotion_recognition_valence}
\end{figure}

% real vs. fake
\begin{figure}[t]
     \centering
     \subfigure{\includegraphics[height=0.3\textwidth]{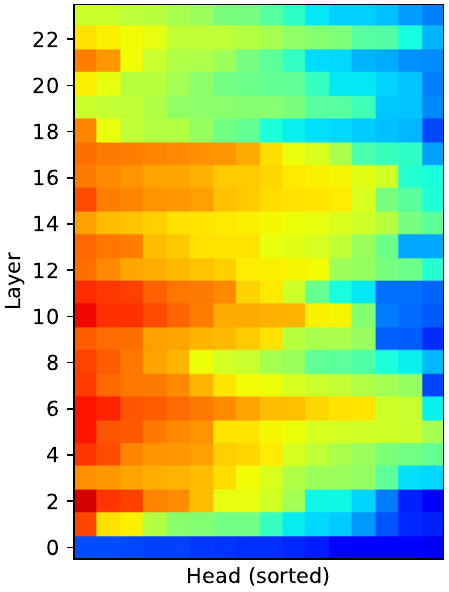}}
     \hfill
     \subfigure{\includegraphics[height=0.3\textwidth]{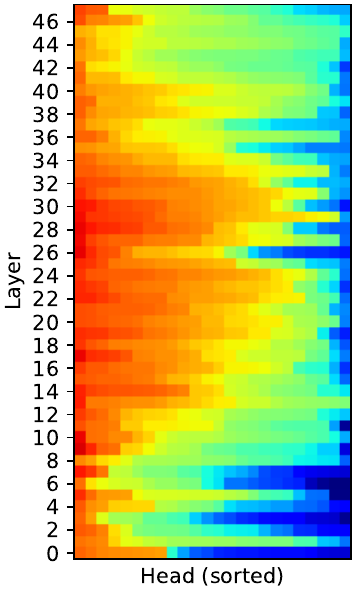}}
     \hfill
     \subfigure{\includegraphics[height=0.3\textwidth]{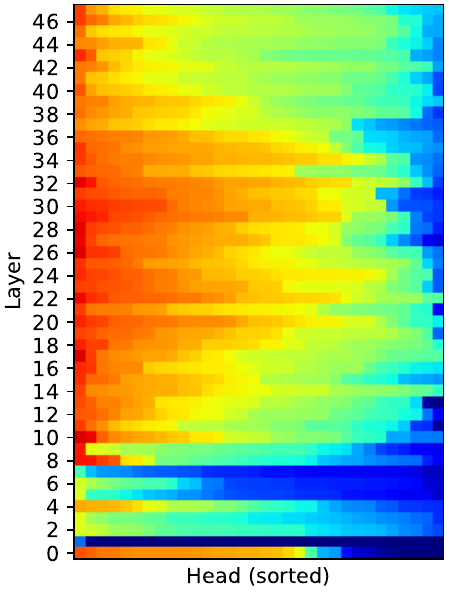}}
     \hfill
     \subfigure{\includegraphics[height=0.3\textwidth]{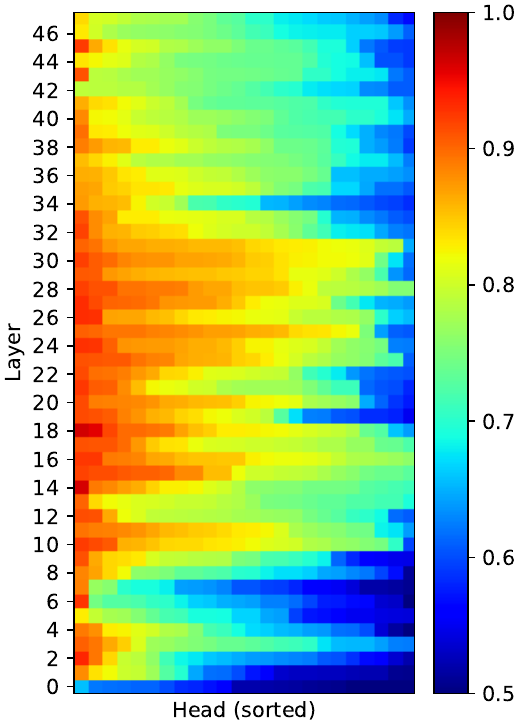}}
     \setcounter{subfigure}{0}
     \subfigure[MusicGen$_\text{small}$]{\includegraphics[width=0.24\textwidth]{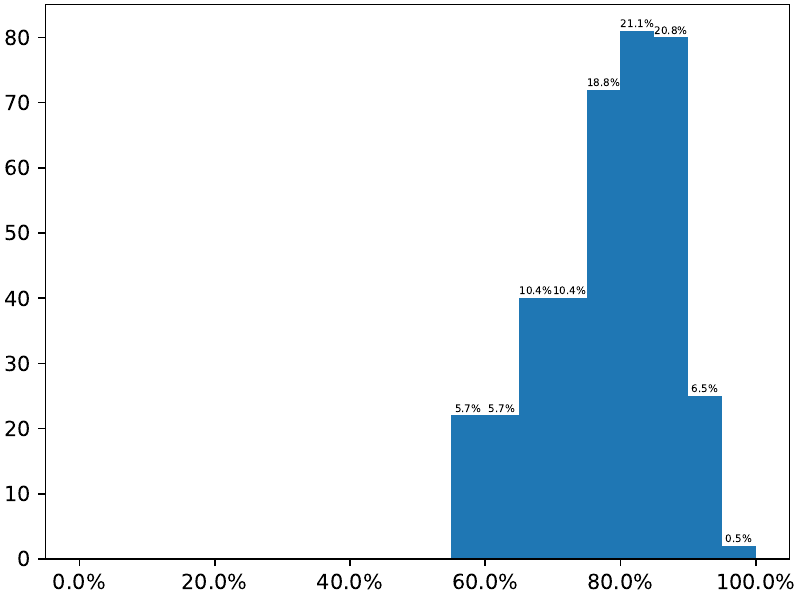}}
     \hfill
     \subfigure[MusicGen$_\text{medium}$]{\includegraphics[width=0.24\textwidth]{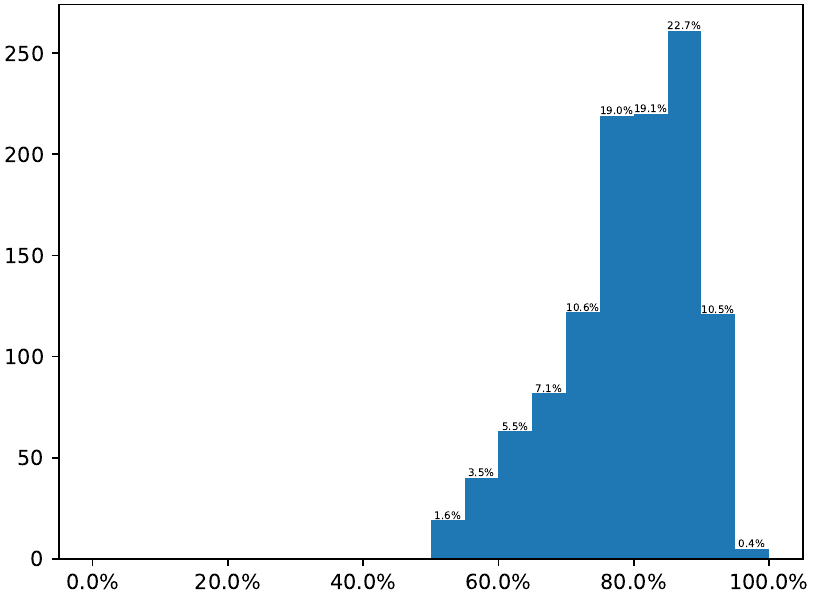}}
     \hfill
     \subfigure[MusicGen$_\text{large}$]{\includegraphics[width=0.24\textwidth]{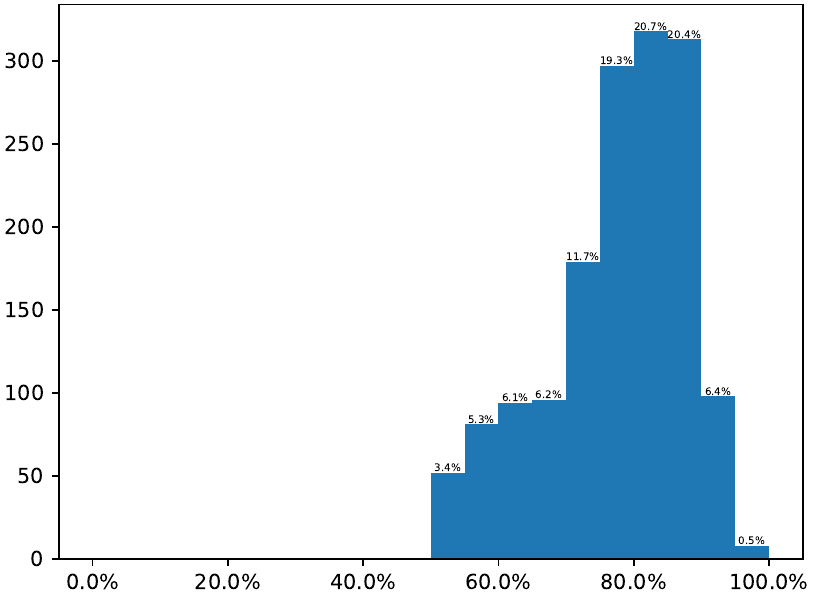}}
     \hfill
     \subfigure[MusicGen$_\text{melody}$]{\includegraphics[width=0.24\textwidth]{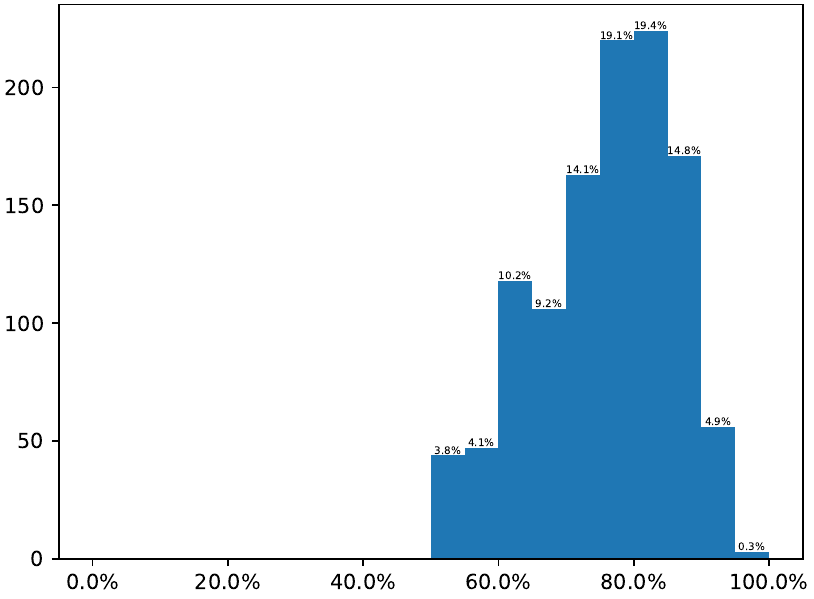}}
     \caption{Probe accuracy and its histogram for real vs.\ fake music}
    \label{fig:probe_acc_real_fake}
\end{figure}
