# Supplementary material for: SMITIN: Self-Monitored Inference-Time INtervention for Generative Music Transformers
Source: arXiv:2404.02252 source file (2025-02-01)
Supplement: Supplementary file 2 [file obj_eval_appendix_num_data.tex]

\begin{table*}[t]
\centering
\sisetup{
    detect-weight,
    mode=text,
    tight-spacing=true,
    round-mode=places,
    round-precision=3,
    table-format=1.3,
    table-number-alignment=center
    }
    % \vspace{-.24cm}
\caption{
    % Effects on Number of Probing Data - Full Results ($^*$shows full-set success rate) % ICML
    Effects on Number of Probing Data ($^*$shows full-set success rate)
}
\setlength\tabcolsep{3.5pt}
\footnotesize
\resizebox{1.0\linewidth}{!} {
\begin{tabular}{
    l
    S[round-precision=1,table-format=2.1]
    S[round-precision=1,table-format=2.1]
    S[round-precision=1,table-format=2.1]
    S[round-precision=1,table-format=2.1]
    S[round-precision=1,table-format=2.1]
    c*{9}{S}
    S[round-precision=1,table-format=2.1]
    S[round-precision=1,table-format=2.1]
    S[round-precision=1,table-format=2.1]
    S[round-precision=1,table-format=2.1]
    S[round-precision=1,table-format=2.1]
}
\toprule

 \multirow[b]{2.55}{*}{\shortstack[t]{\textbf{Number of}\\\textbf{Paired Data}}   }  & \multicolumn{5}{c}{\textbf{Success Rate* [\%] ($\uparrow$)}}                                       & \multicolumn{5}{c}{\textbf{FAD$_\text{L-CLAP mus}$ ($\downarrow$)}}  &  \multicolumn{5}{c}{\textbf{Similarity ($\uparrow$)}} & \multicolumn{5}{c}{\textbf{Probes Max. Acc [\%] ($\uparrow$)}}  \\ 
\cmidrule(lr){2-6}\cmidrule(lr){7-11}\cmidrule(lr){12-16}\cmidrule(lr){17-21}
& \textit{drums} & \textit{bass} & \textit{guitar} & \textit{piano} & \textit{avg.} & \textit{drums} & \textit{bass} & \textit{guitar} & \textit{piano} & \textit{avg.} & \textit{drums} & \textit{bass} & \textit{guitar} & \textit{piano} & \textit{avg.} & \textit{drums} & \textit{bass} & \textit{guitar} & \textit{piano} & \textit{avg.} \\ 
\midrule
\textbf{$n$ = 10} & 28.3 & 42.9 & 48.4 & 4.5 & 31.0 & 0.344 & 0.267 & 0.445 & 0.373 & 0.357 & 0.855 & 0.928 & 0.920 & 0.935 & 0.909 & 88.6 & 85.3 & 73.3 & 69.0 & 79.1\\
\textbf{$n$ = 100} & 25.0 & 48.9 & 45.0 & 8.3 & 31.8 & 0.368 & 0.289 & 0.406 & 0.336 & 0.349 & 0.866 & 0.920 & 0.929 & 0.941 & 0.914 & 91.6 & 87.8 & 78.3 & 72.8 & 82.6\\
\textbf{$n$ = 500} & 24.5 & 41.0 & 38.2 & 5.8 & 27.3 & 0.360 & 0.280 & 0.395 & 0.330 & 0.341 & 0.865 & 0.923 & 0.934 & 0.940 & 0.915 & 93.6 & 88.8 & 81.0 & 74.1 & 84.4\\
\textbf{$n$ = 1000} & 25.1 & 37.6 & 34.1 & 5.5 & 25.5 & 0.357 & 0.273 & 0.400 & 0.331 & 0.340 & 0.861 & 0.927 & 0.930 & 0.940 & 0.914 & 94.3 & 89.1 & 81.4 & 74.7 & 84.8\\
\cdashlinelr{1-21}
\textbf{$n$ = full} & 20.6 & 30.4 & 33.8 & 8.7 & 23.3 & 0.346 & 0.267 & 0.397 & 0.337 & 0.336 & 0.857 & 0.922 & 0.935 & 0.938 & 0.913 & 94.3 & 89.1 & 81.8 & 75.3 & 85.1\\
\bottomrule
\end{tabular}
}
% \vspace{-5pt}
\label{tab:num_data_full}
\end{table*}
